# Supplementary material for: ALEX: Towards Effective Graph Transfer Learning with Noisy Labels
Source: arXiv:2309.14673 source file (2023-09-26)
Supplement: Supplementary file 1 [file 7_appendix.tex]

% \clearpage

\section{Details of datasets}

% 这是正文
% Benchmark Datasets. In this experiment, we diligently assess
% the performance of our proposed model by examining it on three
% real-world networks sourced from ArnetMiner [37]. The networks
% are constructed based on paper citation information obtained from
% various databases, namely DBLP, ACM, and Microsoft Academic
% Graph. Detailed dataset information is presented in Table 1.
% Since all labels in the datasets are clean, following [6, 28, 53],
% we employ two different disturbance methods to add noise to the
% training labels of the original datasets. (i) Uniform Noise: Label of
% each node is randomly switched to another class with certain probability.
% (ii) Pair Noise: Label of each node is changed exclusively to
% its most similar class with certain probability. In both two methods,
% the probability is a parameter set to 20% by default. To appropriately
% choose the best model and assess its performance, we split
% the dataset into training, testing, and validation sets, maintaining a
% 7:2:1 proportion for each respective set.
% Evaluation Protocols. To evaluate our algorithm

In this part, we introduce dataset processing details and feature extraction methods. The first data group: 1A and 1D (ACMv9 and DBLPv8) contain papers published between 2000 and 2010 and after 2010 respectively. The labels of each paper are determined by six categories according to its research area, including “Database”, “Data mining”, “Artificial intelligent”, “Computer vision”, “Information Security” and "High-Performance Computing". As for the second group: 2A, 2D, 2C (ACMv9, DBLPv7, and Citationv1), they are also published in different periods, i.e., 
after 2010, between 2004 and 2008, and before year 2008. Each paper is labeled according to one of
the following five categories,
including “Databases”, “Artificial Intelligence”, “Computer
Vision”, “Information Security”, and “Networking”.
In our studies, we view these datasets as non-directional networks, with each edge representing a citation connection between two academic papers.

% for each dataset, we extracted the
% papers published in different periods, i.e., DBLPv8 (after year 2010),
% ACMv9 (between years 2000 and 2010), and Citationv2 (before year
% 2008). In our experiments, we consider them as undirected networks
% and each edge representing a citation relation between two papers.
% We classify papers into some of the following 

% six categories according
% to its research topics, including “Database”, “Data mining”, “Arti-
% ￿cial intelligent”, “Computer vision”, “Information Security” and
% "High Performance Computing". 
% We evaluate our proposed model
% by conducting multi-label classi￿cation on these three network
% domains through six transfer learning tasks including C!D, A!D,
% D!C, A!C, D!A, and C!A, where D, A, C denote DBLPv8,
% ACMv9 and Citationv2, respectively

\section{Details of baselines}
We compare \method{} with methods including state-of-art Single-domain and  Cross-domain node classification models. Their details are elaborated as follows:

\noindent\textit{Single-domain node classification models}. These models have not been subjected to cross-domain training. We first train and validate them on source data, then test them on the target dataset.

\begin{itemize}[leftmargin=*]
    \item   MLP: This method ignores graph information. We use the MLP encoder structurally consistent with DGRL to ensure fairness.
  \item DeepWalk~\cite{perozzi2014deepwalk}: A technique for compressing node representations based on the Skip-Gram model, using a random walk sampling strategy to determine the neighborhood of each node.
  \item GraphSAGE~\cite{hamilton2017inductive}: A method generating embedding by sampling and aggregating features from a node’s local neighborhood.
  \item LINE~\cite{tang2015line}: A method optimizing a meticulously crafted objective function in order to maintain both the local and global structures of the graph.
  \item GCN~\cite{kipf2017semi}: A graph neural network inspired by Convolution Neural Network to aggregate information from neighboring nodes.
\end{itemize}

\noindent\textit{Cross-domain node classification models}. These models are designed to have strong generalization capabilities and undergo cross-domain optimization during training.

\begin{itemize}[leftmargin=*]
    \item DGRL~\cite{ganin2016domain}: This model utilizes a 2-layer MLP as a feature generator to obtain node representations, and utilizes gradient reverse layer (GRL) for subsequent domain classification. It is a foundational work in the domain adaptation field.
    \item AdaGCN~\cite{dai2022graph}: This model is similar to DGRL with a base classifier and GRL domain classifier, but the feature generator employs a GCN architecture.
    \item UDAGCN~\cite{wu2020unsupervised}: This model utilizes a dual graph convolutional network component and attention mechanism for more effective graph representation. 

\end{itemize}

\section{Other Details}
In our machine learning research, we leverage advanced tools and hardware to achieve optimal results. Our toolkit primarily consists of Python-based libraries, specifically PyTorch 1.11.0 and PyTorch Geometric 2.11.0.  Besides, we employ all experiments on NVIDIA A40 to ensure high-speed computation. For \method{}, GCN, AdaGCN, and UDAGCN, we use two hidden GCN layers with 128 \& 16 hidden dimensions respectively. MLP and DGRL adopt the same linear layers with the same number of hidden dimensions. All hyper-parameters are tuned based on the validation set for a fair comparison. For our \method{}, we vary $q$ and $\alpha$ among $\{200, 300, 400, 500, 600\}$ and $\{70, 75, 80, 85, 90\}\%$ and find best model by grid search. The label noise rates are tuning from $\{0, 10, 20, 30, 40\}\%$ with details in Sec 4.3 and set to 20\% by default. All models share a learning rate of $1 e-4$ with Adam optimizer.
